# Supplementary material for: Triplet supercurrents in lateral Josephson junctions with a half-metallic ferromagnet
Source: arXiv:2303.13922 source file (2024-10-09)
Supplement: Supplementary file 1 [file LSMO_disk_SI_revised_sep24.pdf]

# Triplet supercurrents in lateral Josephson junctions with a half-metallic ferromagnet

Yao Jungxiang,*,† Remko Fermin,† Mariona Cabero Piris,‡ Kaveh Lahabi,† and Jan Aarts*,†

†*Huygens-Kamerlingh Onnes Laboratory, Leiden University, P.O. Box 9504, 2300 RA Leiden, The Netherlands.*

‡*ICTS - Centro Nacional de Microscopía Electrónica, Universidad Complutense de Madrid, 28040 Madrid, Spain*

E-mail: yao@physics.leidenuniv.nl; aarts@physics.leidenuniv.nl

## I Characterization of the epitaxy of LSMO films

LSMO films with a thickness of 40 nm were grown on LSAT substrates in an off-axis sputtering system. We employed different methods to examine and characterize the epitaxy of LSMO. Atomic force microscopy (AFM) was used to map the morphology of the films. As shown in Fig.S1a, clear atomic terraces were observed. Furthermore, x-ray diffraction (XRD) was used to verify the epitaxial growth of LSMO free of crystalline defects (Fig.S1b). Also, we measured the temperature-dependent resistivity of LSMO films using a Van de Pauw method. By calculating the temperature derivative of resistivity, The Curie temperature ($T_c$) was determined to be $\sim$ 362 K (inset in Fig.S1c), consistent with the bulk value. The magnetic properties were measured by vibrating sample magnetometry (Fig.S1d). The coercive field was about 2.5 mTe, and the saturation magnetization was calculated to be $\sim$ 3.8 $\mu_B/f.u.$, in agreement with the theoretical value. Therefore, we conclude that the LSMO

films used inthis work are of high quality.

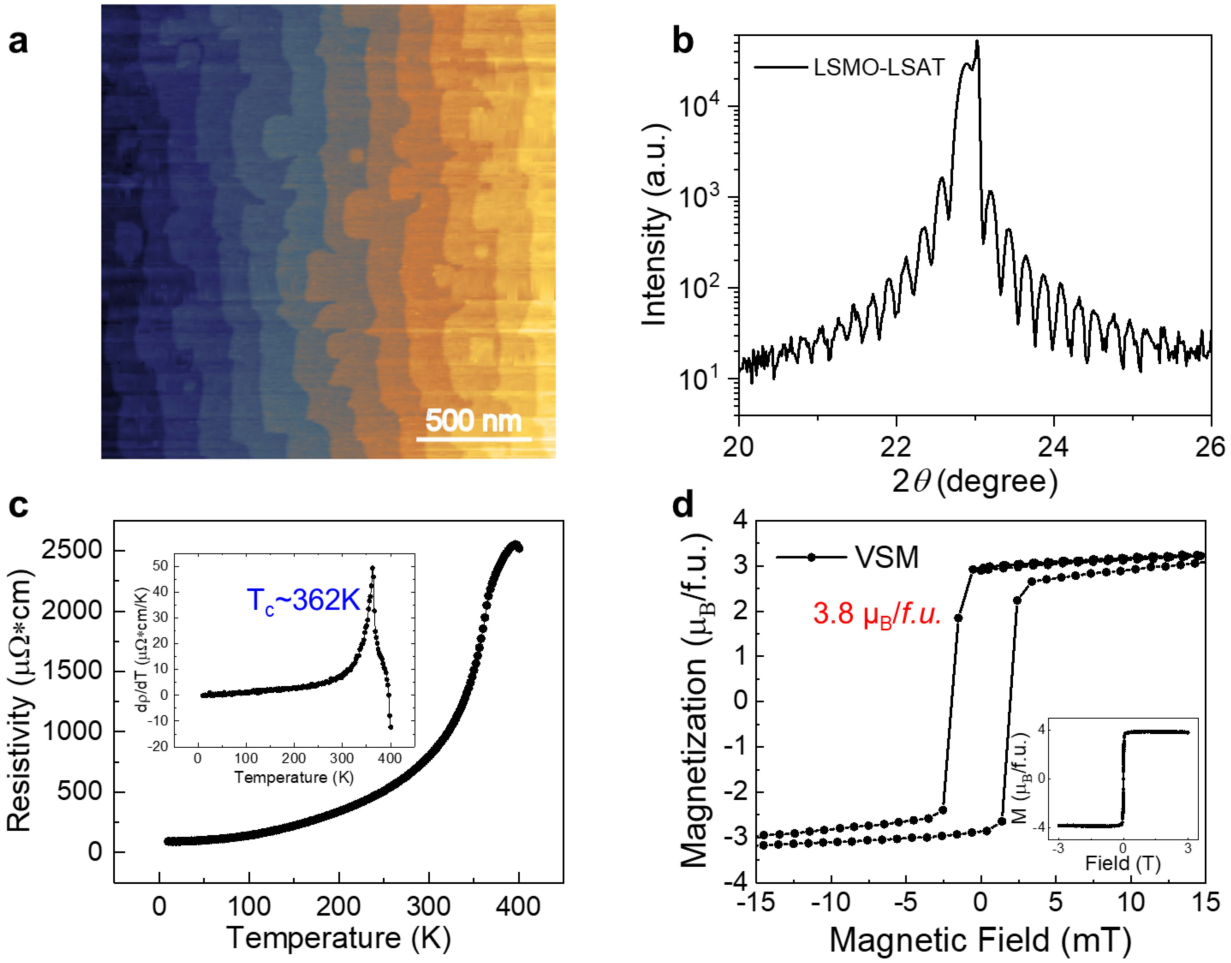


**Figure S1.** Property of epitaxial LSMO film. (a) AFM image of morphology of LSMO film. (b) XRD analysis at low-angel region. (c) Temperature-dependent resistivity characteristics. The inset shows the temperature derivative of resistivity to determine the Curie temperature $T_c \sim 362$ K. (d) Magnetization *vs* field curve obtained at 50 K. The inset is the full-range measurement with a field up to 3 T.

## II Junctions with shallow and deep trenches; and the 5:1 bar

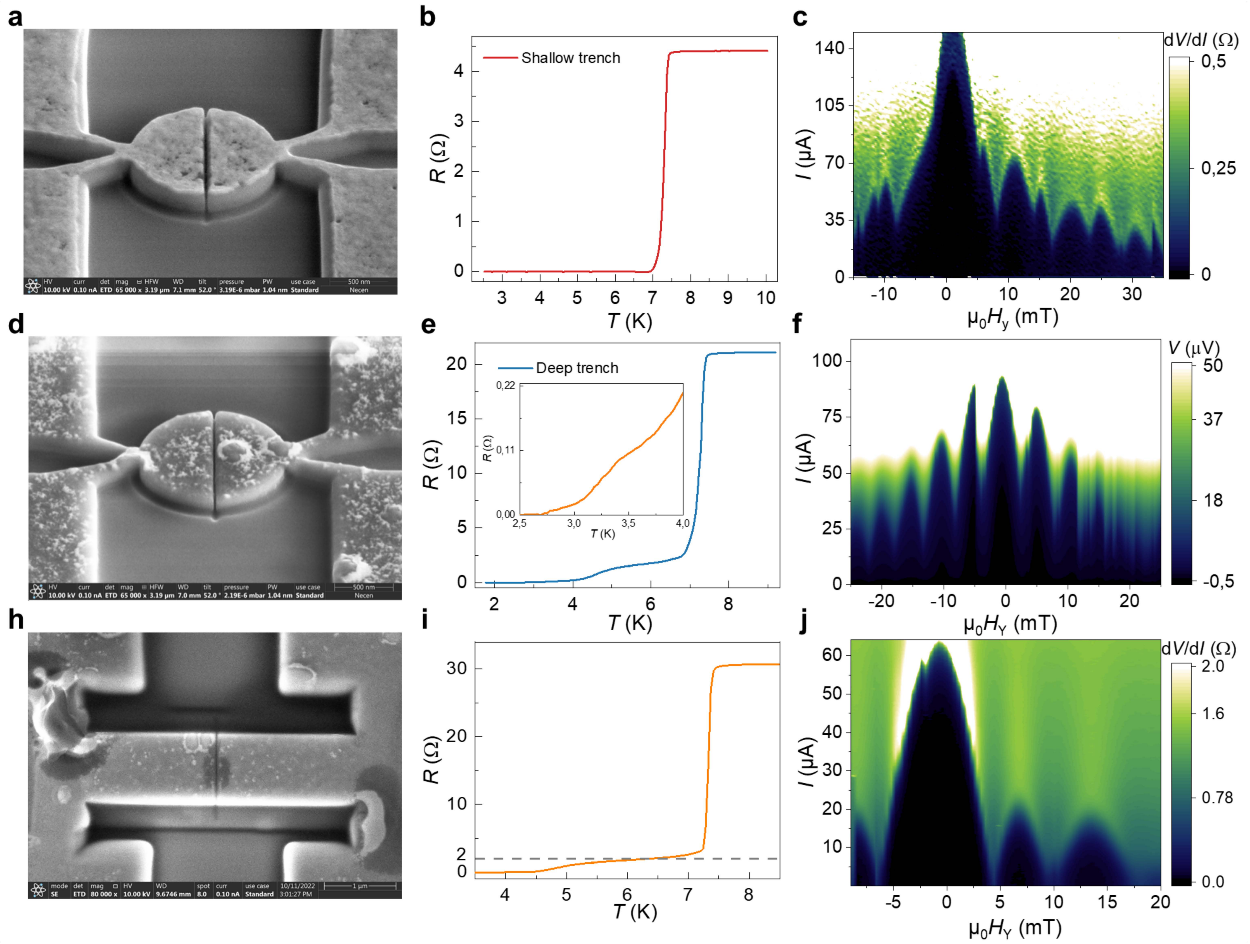


**Figure S2.** Characterizing NbTi/LSMO junctions with shallow and deep trenches. Front-view of SEM images of junctions with shallow (a) and deep (d) trenches. (b) and (e) corresponding RT curves. The inset in (e) is the magnification of the low-temperature region to clarify the second transition temperature. At 5.5 K, the measured SQI pattern of the junction with a shallow trench is Fraunhofer-like, while the junction with a deep trench exhibits a SQUID-like SQI pattern at 2.5 K, indicating rim supercurrents only appear in a disk-shaped ferromagnetic weak link. Note that a shallow trench means the weak link is NbTi. (h) SEM image of the bar-shaped junction with an aspect ratio 5:1, and (i) the measured RT of this junction. (j) The obtained SQI pattern is Fraunhofer-like at 3.2 K, in agreement with the observation on the bar-shaped (3:1) junction in the main text.

# III Analyzing SQI patterns

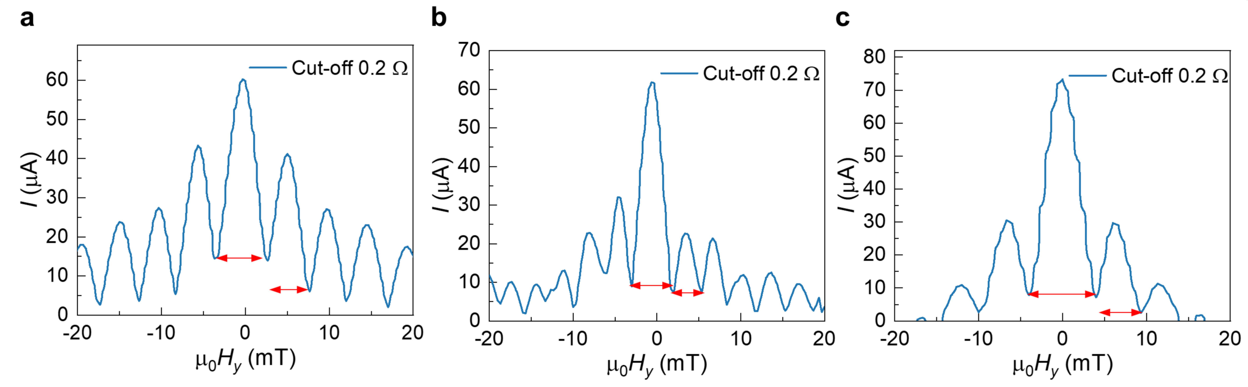


**Figure S3.** Plot of the extracted critical current with a resistance criterion for the disk-shaped (a), square-shaped (b), and bar-shaped (c) NbTi/LSMO junctions, corresponding to Fig.3 in the main text.

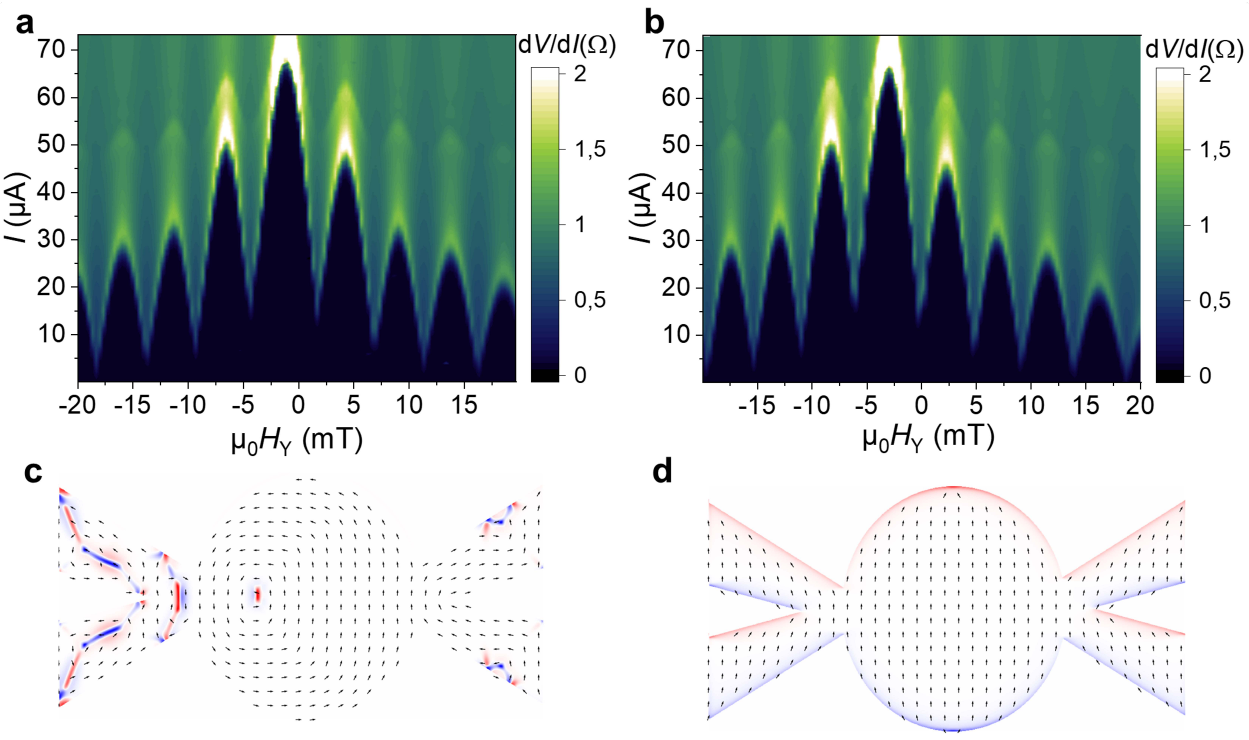


**Figure S4.** Measured SQI patterns with constant IP field 10 mT (a) and 100 mT (b) along the trench at 4.1 K. No change in both the amplitude and period of the SQI patterns is observed. The shift of the central peak with respect to the zero field is due to the misalignment between the sample and IP fields. (c) and (d) are the simulated magnetization states, correspondingly.

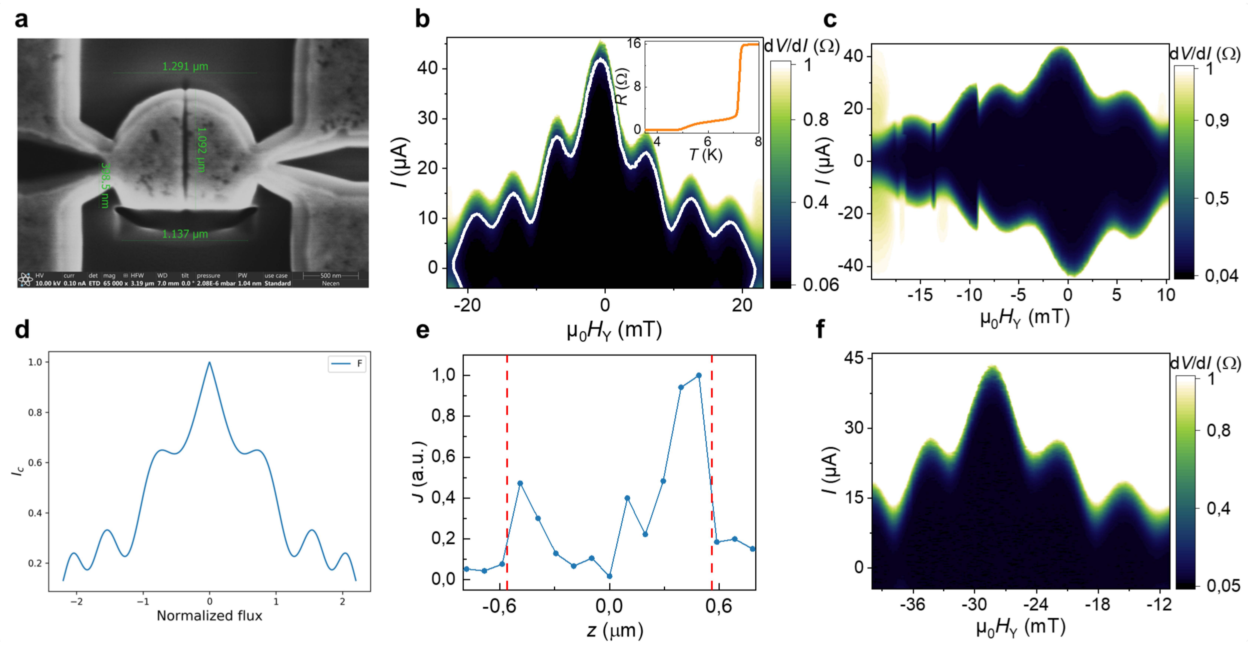


**Figure S5.** (a) Top-view SEM image of a disk with a flat side. (b) SQI pattern of this irregular disk, measured at 4.1 K. The white curve is the plot of the critical current that is extracted with a resistance criterion of 0.2 Ω. The inset shows the RT curve of the junction. (c) SQI pattern with sweeping current positively and negatively. (d) Simulated critical current as a function of magnetic flux quanta. (e) Fourier analysis on the SQI pattern in (b) taken with the resistance criterion. (f) SQI pattern in the presence of an in-plane (IP) field of 200 mT.

# IV A disk-shaped NbTi/LSMO junction with a flat side

Having seen no effect of the IP fields on the triplet supercurrents (Fig.4 in the main text), we reshape the LSMO disk, after having performed the measurements presented in the main text, by cutting off one side and thus acquire an irregular geometry of the LSMO-based junction (Fig.S5). Consequently, the pure magnetic vortex will not be the ground state, and local stray fields can occur. In Fig.S5b, the obtained SQI pattern becomes quite abnormal with non-zero minima. By determining both the positive and the negative critical current, we see that the SQI pattern is asymmetric (Fig.S5c). Moreover, the ratio between the period of the central peak and that of the first lobe has increased significantly, to $\sim 1.59$.

Börcsök *et al.*[1] modeled the complex Fraunhofer patterns arising from a non-homogeneous magnetization inside the barrier, in particular when it is larger at the edges of a magnetic Josephson junction. Using Eq. 9 in Ref,[1] we show a qualitative calculation in Fig.S5d with $p$ = 0.2, $Q$ = -1, and $q$ = 3, though a quantitative fitting is not obtained due to the irregular geometry of this junction. The simulated curve is analogous to the measured critical current upon the out-of-plane field (the white curve in Fig.S5b). Interestingly, we still see rim supercurrents on one side in this case. On the other side, the rim supercurrents are largely suppressed, according to the Fourier analysis(Fig.S5e). We again apply IP fields ($\sim$ 200 mT) to saturate the magnetization of this junction. As shown in Fig.S5f, the measured SQI pattern does not change, indicating the transport of triplet supercurrents is intrinsic in the variously shaped NbTi/LSMO junctions, regardless of the magnetization states.

# V Inserting a Ag layer at the LSMO/NbTi interface

Fig. S6 shows measurements on a device where 10 nm of Ag was deposited on LSMO, before growing the NbTi layer. The data are basically indistinguishable from those on devices without the Ag layer, with similar critical currents and SQI patterns. Again, the disk-shaped device shows a SQUID-like pattern, the bar-shaped device a Fraunhofer one.

The reason for the similar behavior becomes clear from the STEM HAADF image shown in Fig. S7. the LSMO is flat over long lateral distances, while the Ag layer grows in Volmer-Weber mode (3D), leading to Ag islands every 150-300 nm. The triplet generator, presumably present at the LSMO/NbTi interface, is clearly not influenced.

# VI Averaged EEL chemical map of the LSMO/NbTi interface

Figure S8a displays a high angle annular dark field image showing the high quality LSMO layer and the disordered LSMO/NbTi interface. Figure S8b shows a chemical profile of the layers from an averaged electron energy loss spectrum image, measured by the normalized intensities at the ionization edges of La M4,5, Mn L2,3, Nb L2,3, O K, Sr L2,3 and Ti L2,3. The interface is quite sharp, with no significant intermixing, although a few atomic layers around the interface may well be a mixture of La, Sr, Mn, Nb and Ti. What stands out is a small peak in the oxygen concentration that we found in two out of three samples.

# VII Determining $I_c$ and calculating $E_{Th}$

Raw $IV$ curves are given in Fig. S9a. At high temperatures, all $IV$ curves have pronounced rounding features at $I \sim I_c$ due to phase slippage, leading to ambiguity in determining $I_c$.[2] Following Ambegaokar and Halperin,[3] we calculate the IV curves analytically giving

$$V = \frac{2I_c R_N}{\gamma_0} \frac{e^{\pi\gamma_0 i} - 1}{e^{\pi\gamma_0 i}} \left\{ \int_0^{2\pi} e^{-i\gamma_0\varphi/2} I_0(\gamma_0 sin\frac{\varphi}{2}) d\varphi \right\}^{-1} \tag{1}$$

where $\gamma_0 = \Phi_0 I_c/\pi k_B T$, $i = I/I_c$. $I_c$ is the critical current, $R_N$ is the normal resistance, $I_0$ represents a modified Bessel function. The simulated results are shown in Fig.S9b. As $\gamma_0$ becomes large enough, meaning the Josephson coupling energy is comparable to the thermal energy, the rounding feature is significantly suppressed. Shifting the baselines of the $IV$ curves to zero by subtracting the minimum of each $IV$ curve individually, we then fit the measured $IV$ to Eq1 and determine $I_c$ analytically (Fig.S9c). We obtain an average $R_N \approx 0.8\ \Omega$. The fitted $I_c$ is slightly larger than the extracted $I_c$ with a resistance criterion.

Next, we discuss the $I_c$ versus temperature. In the main text, we argued that a description that assumes the diffusive and long regime of a mesoscopic junction, such as used in Refs.,[4–6]

is not valid. Here, a diffusive and long junction means $\ell_H < d$ and $\Delta > E_{Th}$. Unlike the YBCO/LSMO system, in which $k_B T \gg E_{Th}$,[6] the second transition temperature of the NbTi/LSMO junction is quite low $\sim 5.2\ K$. First we therefore fit the temperature dependence of $I_c$ to Eq. 1 in the low-temperature limit ($k_B T \ll E_{Th}$), according to Ref,[5]

$$\frac{eR_N I_c}{E_{Th}} = a(1 - be^{-aE_{Th}/3.2k_B T}) \tag{2}$$

where the coefficients a and b are 10.82 and 1.30, respectively. $k_B$ is the Boltzmann constant, and $T$ represents temperature. The result of the fit is shown in Fig. S9d (cyan line) and at first sight looks good. However, the resulting $E_{Th} \approx 34.6\ \mu$eV, is much smaller than $k_B T$ ($\sim$ 353 $\mu$eV at 4.1 K). The fitted $R_N$ is 0.37 Ω and unreasonable, in view of both the residual resistance in the RT curve (Fig.2 in the main text) and the fitted data with the AH theory.

Therefore, we consider the high-temperature case (k$_B T \gg E_{Th}$) and fit the temperature-dependent $I_c$ to

$$eR_N I_c = 64\pi k_B T \sum_{n=0}^{\infty} \frac{L}{L_{\omega_n}} \frac{\Delta^2 \exp^{-L/L_{\omega_n}}}{[\omega_n + \Omega_n + \sqrt{2(\Omega_n^2 + \omega_n \Omega_n)}]^2} \tag{3}$$

where $L$ is the length of the junction ($d$ in the main text), $L_{\omega_n} = \sqrt{\hbar D/2\omega_n}$, $\omega_n = (2n+1)\pi k_B T$ is the Matsubara frequency, $\Omega_n = \sqrt{\Delta^2 + \omega_n^2}$. The fitting curve (magenta) is plotted in Fig. S9d. From this fit, we find $E_{Th}$ to be about 112 $\mu eV$, the fitted $\Delta$ is 788 $\mu eV$, and $T_c$ is 5.27 K. The ratio $E_{Th}/\Delta(0)$ is therefore 0.14. The fitted R$_N$ is about 0.87 Ω, coincident with the fitting results with the AH theory. According to $\Delta(0) = 1.764 k_B T_c$,[7] we obtain $\Delta(0) \approx 790\ \mu eV$, which is in agreement with the fitted $\Delta$. In order to show better what the high-temperature looks like, we simulate the temperature-dependent characteristic $I_c R_N$ voltage based on Eq.3 and plot $I_c$ (in appropriate units) versus $T/T_c$ for various values of $E_{Th}/\Delta(0)$ in Fig. S10. The case of our fit is the green line (a ratio of 0.15), clearly starting off quadratically. The plateau is reached at $T/T_c \approx 0.6$, corresponding to $\sim$ 300 mK in the experiment.

We still argue, however, that this description is unphysical. In the diffusive regime we have $\xi_F = \sqrt{\hbar D/2\pi k_B T_c} \approx 19$ nm with $T_c = 5.5$ K. Therefore, the junction length $d$ nearly equals $\xi_F$. Then, $E_{Th} = \hbar D/L^2 \approx 2.6$ meV, which is clearly larger than $\Delta \approx 0.9$ meV. In other words, there is a strong discrepancy between the calculated (diffusive) value of $E_{Th}$ and the fitted result. We conclude, not surprisingly, that the long diffusive junction limit cannot be valid. Instead, given $\ell_H < d$ and $E_{Th} > \Delta$, we are in the short regime, where our $I_c$ data are (well) well described by $(1 - T/T_c)^2$, as seen in Fig.5 in the main text. Further quantitative analysis of $I_c(T)$ of half-metallic Josephson junction may need rigorous theoretical study.

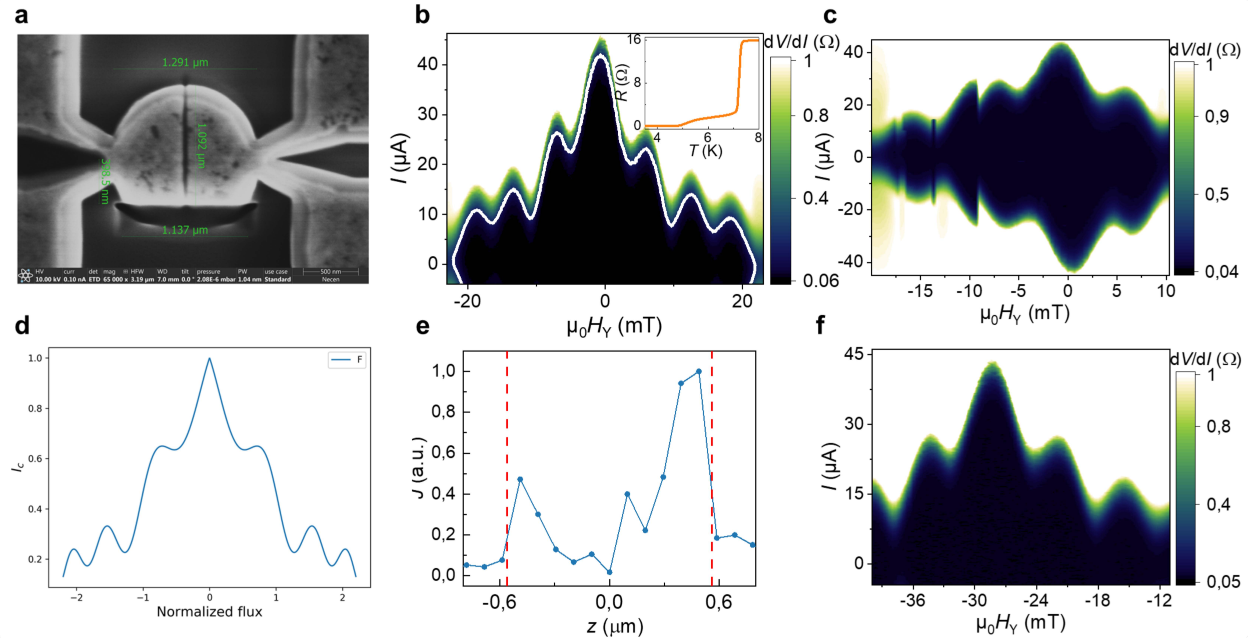


**Figure S6.** (a) RT curves of disk-shaped (blue) and bar-shaped (4:1) (red) NbTi/Ag/LSMO trilayer junctions. The corresponding $I_c(B_\perp)$-patterns, displayed in (b,c) and measured at 4 K, are SQUID-like and Fraunhofer-like, respectively.

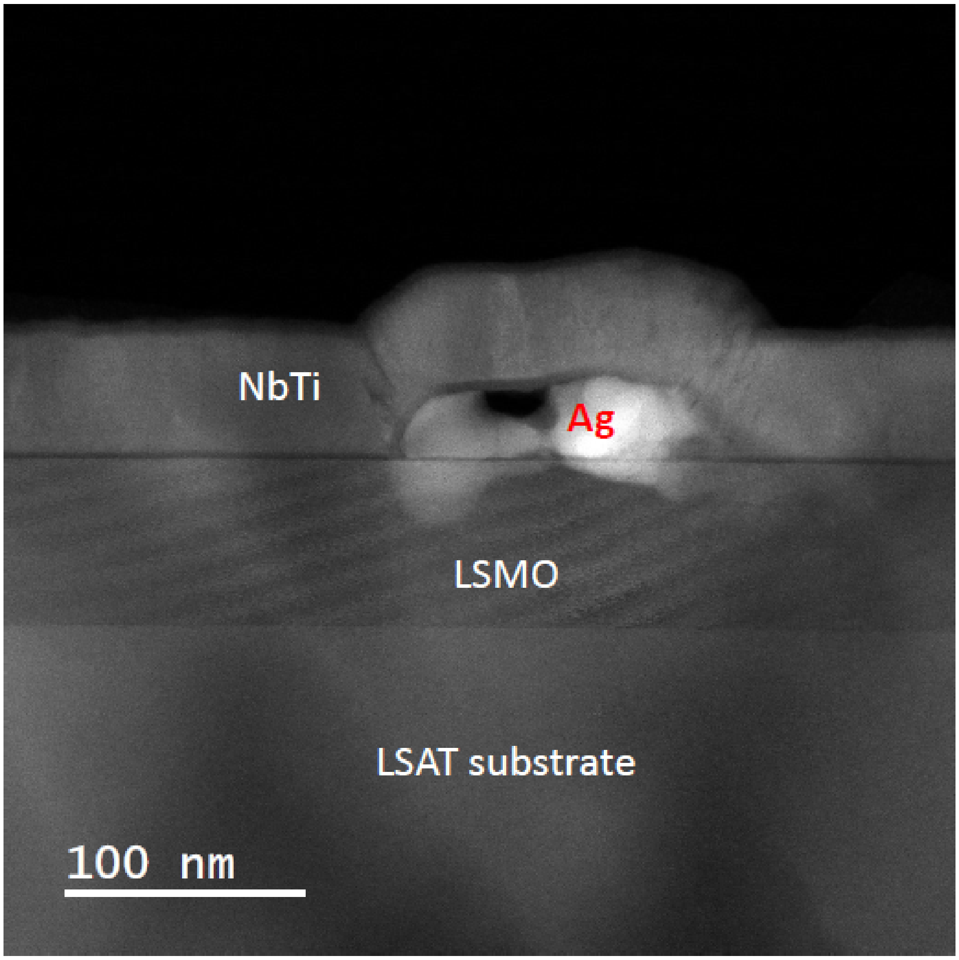


**Figure S7.** Scanning transmission Electron Microscopy image of the LSMO/Ag/NbTi sample grown on LSAT, with the different materials as indicated.

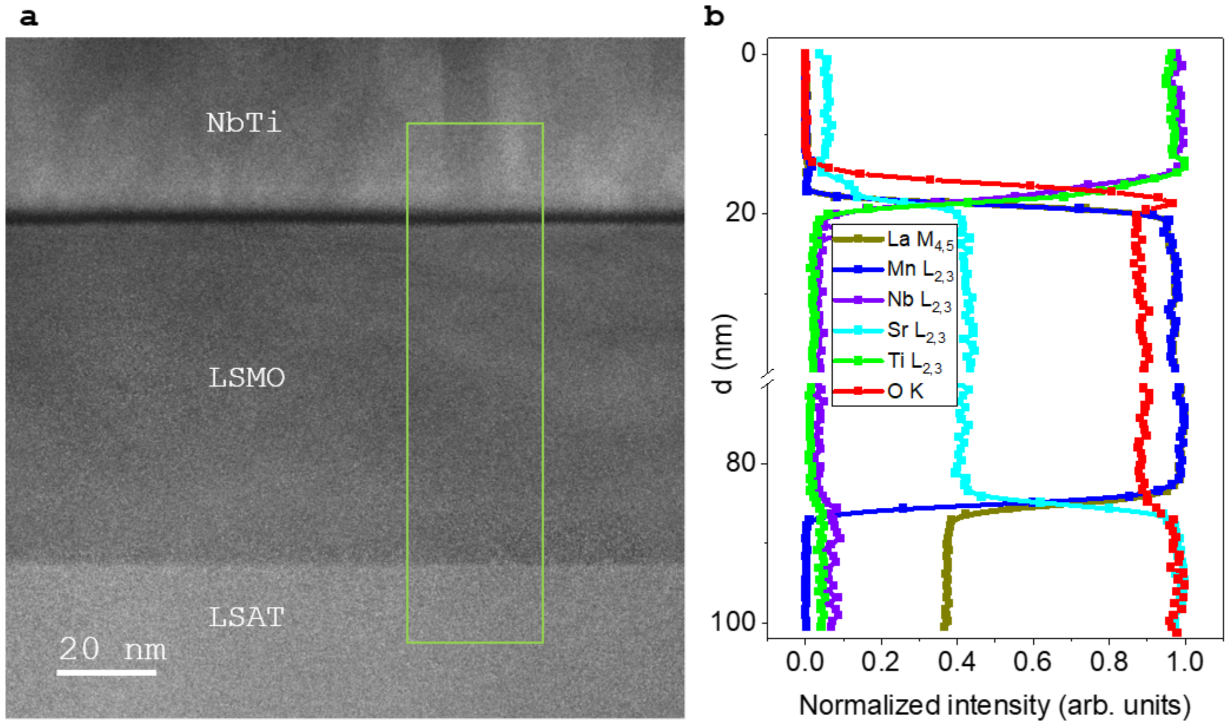


**Figure S8.** (a) High resolution HAADF image of the LSMO/NbTi sample deposited on a (001)-oriented LSAT crystal substrate. The green square marks the zone where an EELS map is obtained for an averaged chemical profile shown in (b). (b) Chemical signals along the interfaces of NbTi/LSMO/LSAT, for the elements as indicated.

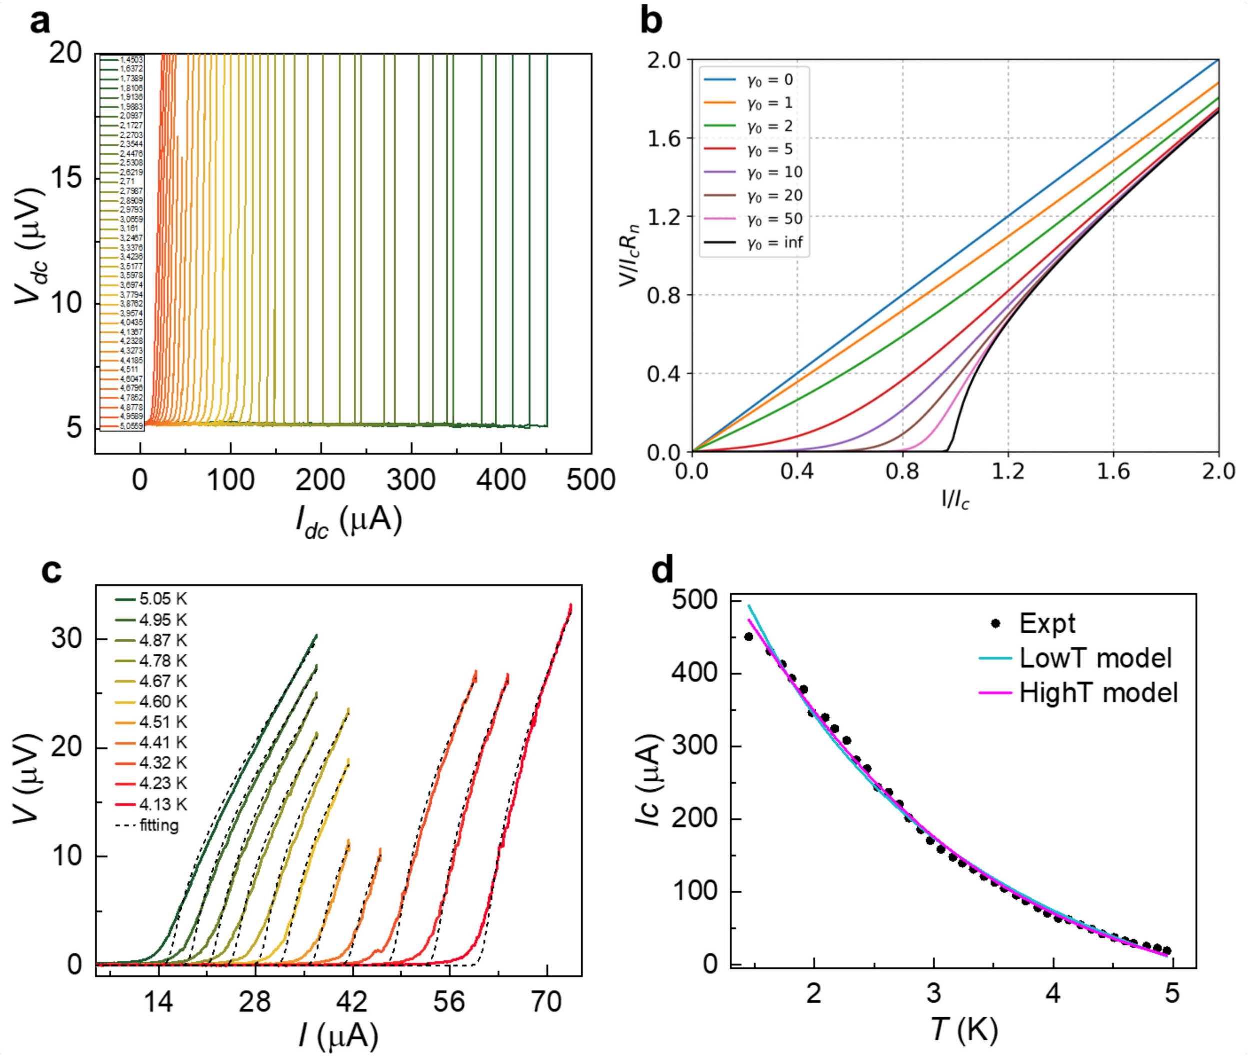


**Figure S9.** Determining $I_c$ and calculating $E_{Th}$. (a) Raw $IV$ curves. (b) Simulated IV curves based on the AH theory, Eq.1, for different values of $\gamma_0 = \Phi_o I_c/(\pi k_B T)$. (c) Measured $IV$ curves at high temperatures and the corresponding fit (black dashed line) using Eq.1. (d) A plot of the fitted $I_c$ as a function of temperature and fits using Eq.2 (cyan curve) and Eq.3 (magenta curve).

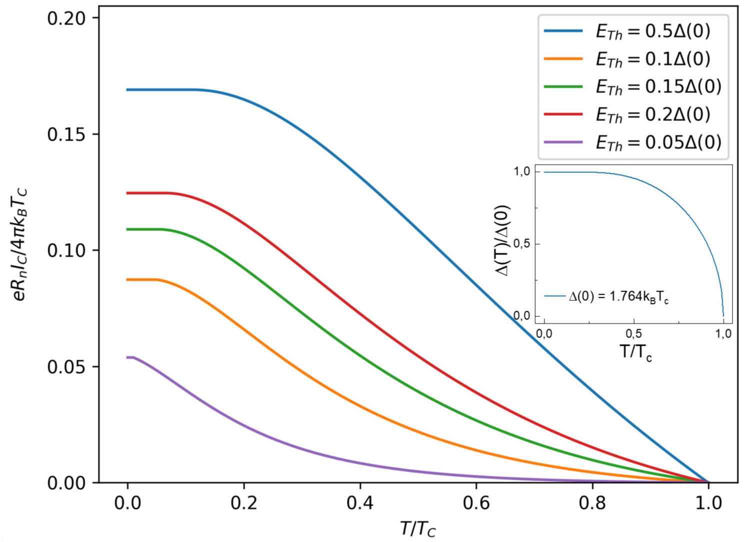


**Figure S10.** Simulated temperature dependence of the product of $eI_cR_N$ at various ratios of $E_{Th}/\Delta(0)$ based on Eq.3. The inset shows the universal $\Delta(T)/\Delta(0)$ as a function of $T/T_c$, in which $\Delta(0) = 1.764k_BT_c$.[7]

# References

(1) Börcsök, B.; Komori, S.; Buzdin, A. I.; Robinson, J. W. A. Fraunhofer patterns in magnetic Josephson junctions with non-uniform magnetic susceptibility. *Sci Rep* **2019**, *9*, 5616.

(2) Blom, T. J.; Mechielsen, T. W.; Fermin, R.; Hesselberth, M. B. S.; Aarts, J.; Lahabi, K. Direct-Write Printing of Josephson Junctions in a Scanning Electron Microscope. *ACS Nano* **2021**, *15*, 322–329.

(3) Ambegaokar, V.; Halperin, B. Voltage due to thermal noise in the dc Josephson effect. *Physical Review Letters* **1969**, *22*, 1364.

(4) Anwar, M. S.; Czeschka, F.; Hesselberth, M.; Porcu, M.; Aarts, J. Long-range supercurrents through half-metallic ferromagnetic $CrO_2$. *Physical Review B* **2010**, *82*.

(5) Dubos, P.; Courtois, H.; Pannetier, B.; Wilhelm, F. K.; Zaikin, A. D.; Schön, G. Josephson critical current in a long mesoscopic S-N-S junction. *Physical Review B* **2001**, *63*.

(6) Sanchez-Manzano, D. et al. Extremely long-range, high-temperature Josephson coupling across a half-metallic ferromagnet. *Nat Mater* **2022**, *21*, 188–194.

(7) Bardeen, J.; Cooper, L. N.; Schrieffer, J. R. Theory of superconductivity. *Physical review* **1957**, *108*, 1175.
